# Supplementary material for: Ultrafast signatures of spin and orbital order in antiferromagnetic $\alpha$-Sr$_2$CrO$_4$
Source: arXiv:2110.14004 source file (2021-10-26)
Supplement: Supplementary file 1 [file supplemental_materials.pdf]

# Supplemental materials for Ultrafast signatures of spin and orbital order in antiferromagnetic $\alpha$ - $\text{Sr}_2\text{CrO}_4$

## I. ASSIGNMENT OF OPTICAL TRANSITIONS IN $\text{Sr}_2\text{CrO}_4$

In our pump-probe measurements, we used pump photon energies of 1.0 eV and 3.1 eV, and 1.55 eV for the probe. We chose these energies based on the calculated partial density of states (PDOS) [1] and experimental optical conductivity data [2]. Based on these references, we display schematic diagrams of spin- and orbital-decomposed PDOS in Fig. S1 for  $T < T_N$ .

First, 1.0 eV photoexcitation induces inter-site hopping between  $d_{zx}$  or  $d_{yz}$  bands at nearest neighbor Cr ions with the same spin polarization. This transition was also observed in optical conductivity ( $\sigma_1$ ) measurements at the same energy of 1.0 eV, for which the intensity saturates at  $T \sim T_N$  with decreasing temperature, as such spin-polarized inter-site hopping is more likely to arise with Néel-type spin order [2].  $T$ -dependent  $\sigma_1$  measurements also reveal a resonant peak at a lower energy of 0.5 eV, consistent with the calculated PDOS [1] showing that this corresponds to inter-site hopping between the same  $d_{zx}$  (or  $d_{yz}$  bands), but with opposite spins, which should be suppressed in the spin-ordered phase, as shown in the experimental data [2].

In addition, from the calculated PDOS, we find resonant energies at  $\sim 3.0$  eV for charge transfer-type transitions from  $O\ 2p$  to  $Cr\ e_g$  states. These energies also correspond to resonant peaks in the experimentally obtained  $\sigma_1$  [2]. For probing the transient reflectivity, we used 1.55 eV photons, below the charge transfer gap energy of 2.0 eV [2], to give general sensitivity to dynamics in all  $t_{2g}$  orbitals.

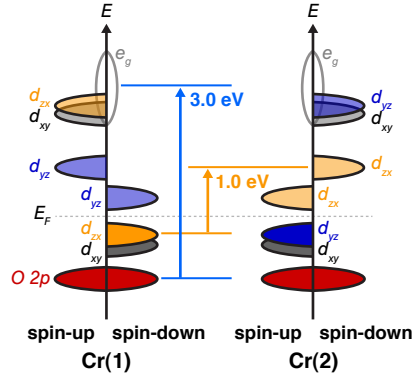

FIG. S1. Spin- and orbital-decomposed partial density of states at nearest-neighbor Cr ions in the antiferromagnetic phase of  $\text{Sr}_2\text{CrO}_4$ .

## II. FITTING THE DATA OBTAINED AFTER 1.0 EV PHOTOEXCITATION

As described in the main text, we fit the transient reflectivity  $\Delta R/R$  at 1.55 eV measured after 1.0 eV excitation to a bi-exponential decay model:

$$\frac{\Delta R}{R}(t) = A_1 \exp\left(-\frac{t}{\tau_1}\right) + A_2 \exp\left(-\frac{t}{\tau_2}\right) \quad (1)$$

where  $A_1$  ( $A_2$ ) and  $\tau_1$  ( $\tau_2$ ) are the amplitude and decay time constants for the fast (slow) dynamics. We plot all of the data and fitting results at different temperatures in Fig. S3. It was not necessary to include a constant parameter in the fitting function.

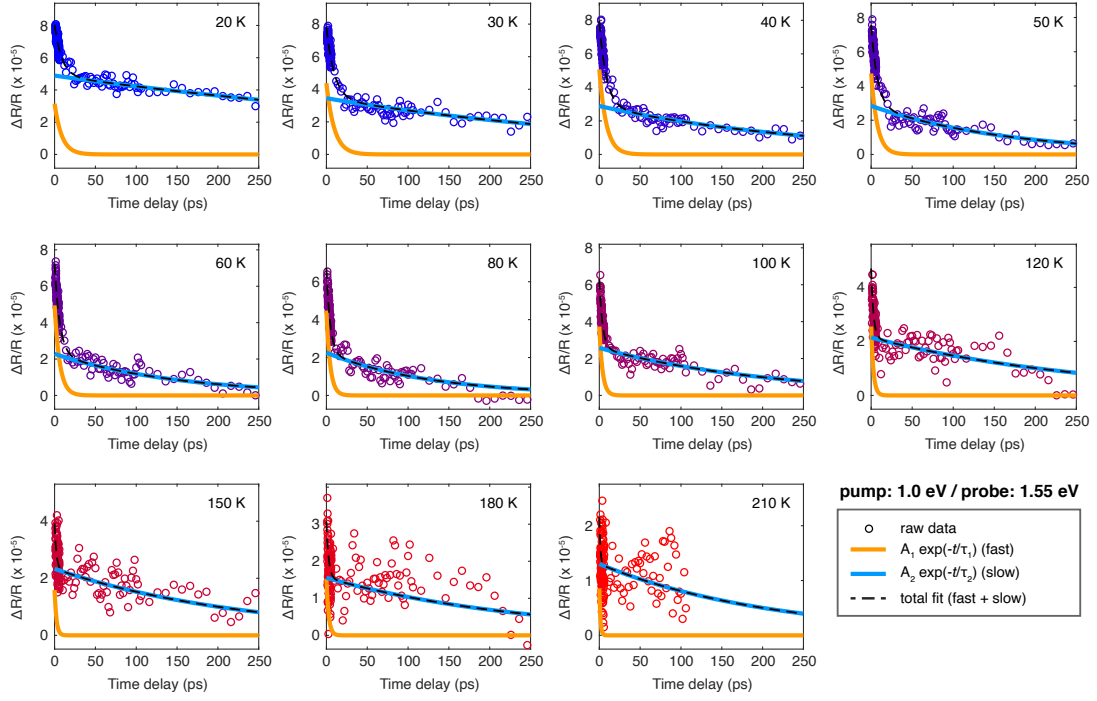

FIG. S2. Transient reflectivity data at various temperatures from 20 K to 210 K (open circles) along with fits using bi-exponential decaying functions (Eq. (1), dashed lines). We also plot specific fast (orange solid line) and slow (sky blue solid line) fit components.

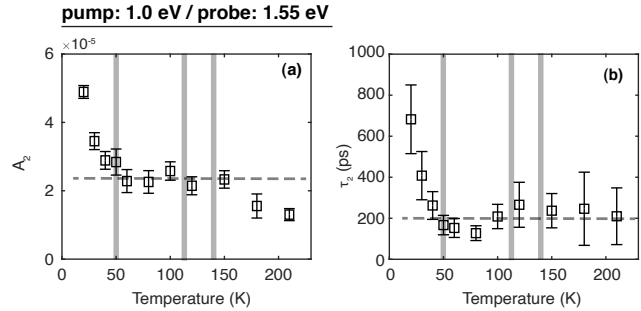

FIG. S3. The temperature dependence of the (a) amplitude  $A_2$  and (d) decay time  $\tau_2$  of the slow component extracted from our fits after 1.0 eV photoexcitation.

### III. FITTING THE DATA OBTAINED AFTER 3.1 EV PHOTOEXCITATION

We were able to use a model based on simple exponential functions to fit only two decay components in our data taken after 1.0 eV photoexcitation, as there was no significant change in the ultrafast rising dynamics with temperature. In contrast, after 3.1 eV photoexcitation, we found a relatively slow rise in the transient reflectivity signal, much longer than the time resolution of our experiments ( $\sim 100$  fs). Therefore, after 3.1 eV photoexcitation,

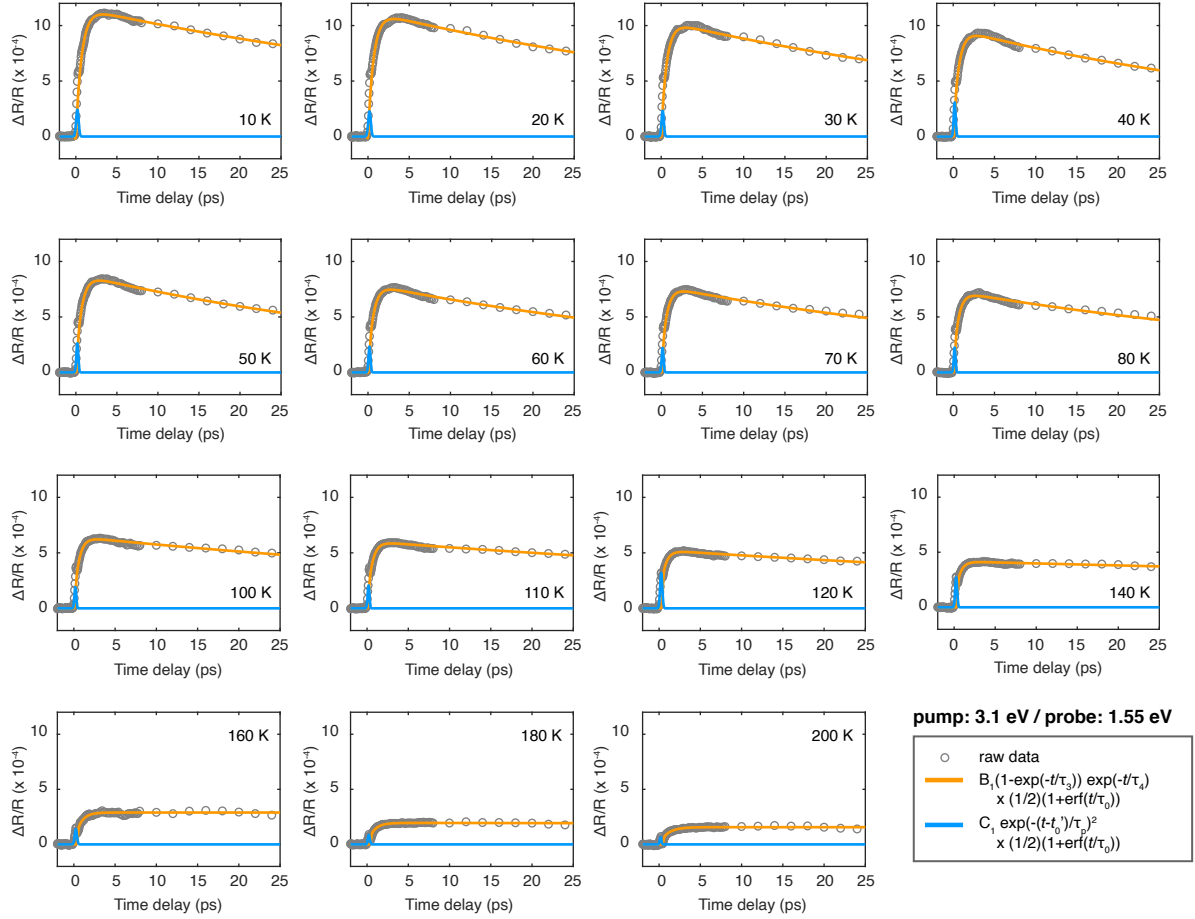

FIG. S4. Transient reflectivity data at various temperatures from 10 K to 200 K (open circles) along with fits using the model described in the text (dashed lines), including a slow rise and consequent decaying dynamics (orange solid lines) as well as a Gaussian-like peak structure (blue solid line).

we fit the transient reflectivity up to 25 ps to a model function given by:

$$\frac{\Delta R}{R}(t) = \frac{1}{2} \left( 1 + \operatorname{erf}\left(\frac{t}{\tau_0}\right) \right) \left( 1 - \exp\left(-\frac{t}{\tau_3}\right) \right) \times \left( B_1 \exp\left(-\frac{t}{\tau_4}\right) + C_1 \exp\left(-\frac{(t - t'_0)^2}{\tau_p^2}\right) \right). \quad (2)$$

In this model, we set a step function  $(1 + \operatorname{erf}(t/\tau_0))/2$  to account for the pulse duration, with fixed  $\tau_0 \sim 100$  fs, and we used  $1 - \exp(-t/\tau_3)$  to fit the slow rising dynamics, while  $B_1 \exp(-t/\tau_4)$  accounts for the consequent relaxation dynamics. We also used a Gaussian-like function,  $C_1 \exp(-(t - t'_0)/\tau_p)^2$ , to fit the initial peak at  $t'_0 \sim 0.2$  ps. We plot the transient reflectivity data and fitting results at various temperatures from 10 to 210 K, as shown in Fig. S4.

Our analysis reveals evidence of the phase transition across  $T_0 = 140$  K from the ultrafast dynamics of the initial peak. As shown in Fig. S5, all fitting parameters, including the amplitude  $C_1$ , peak time  $t'_0$ , and peak width  $\tau_p$ .  $t'_0$  and  $\tau_p$  show  $T$ -dependent anomalies at  $T_N$ , while only  $\tau_p$  changes below  $T_S$ . These anomalies may be due to the fact that both spin and orbital ordering can affect the electronic structure and thus the ultrafast dynamics induced by 3.1 eV photoexcitation.

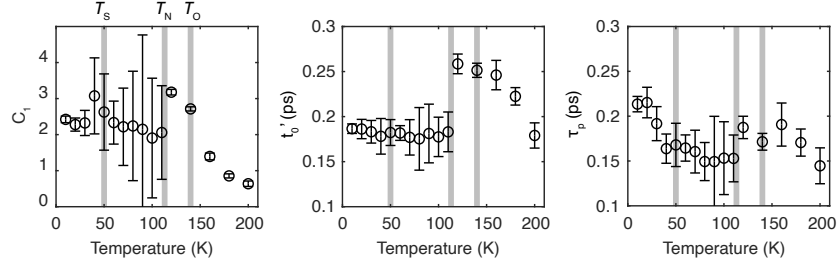

FIG. S5. The amplitude ( $C_1$ ), peak time ( $t'_0$ ) and peak width ( $\tau_p$ ) obtained from the ultrafast dynamics in Fig. S4

#### IV. TEMPERATURE DEPENDENCE OF THE LATTICE PARAMETERS

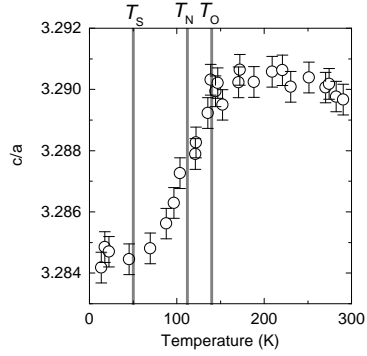

FIG. S6. Temperature dependence of the ratio  $c/a$ , showing a sharp decrease below  $T_O = 140$  K [3]. The three gray lines indicate the transition temperatures for the stripe-type orbital order ( $T_S = 50$  K), Néel-type spin order ( $T_N = 112$  K, and the AF-type orbital order ( $T_O = 140$  K).

#### V. COHERENT ACOUSTIC PHONON OSCILLATIONS

We observed clear coherent phonon oscillations in our 3.1 eV pump/1.55 eV probe measurements, as shown in Fig. S6. We extract the amplitudes and frequencies of the two acoustic phonon modes using a damped harmonic oscillator model:

$$\Delta R_{ap} = \sum_{i=1,2} a_i \exp(-t/\tau_i) \cos(2\pi f_i t - \phi_i). \quad (3)$$

However, we did not find any obvious change across the spin and orbital ordering transitions, except increases in the amplitudes  $a_1$  and  $a_2$  at  $T_O$ , the transition temperature for the antiferro-type orbital ordering described in the main text (Fig. 1(a)). This may be due to a change in the  $c$ -axis lattice parameter, as acoustic longitudinal phonons are sensitive to the out-of-plane crystal structure. This is also consistent with the previous report from neutron scattering experiments [3].

- 
- [1] T. Ishikawa, T. Toriyama, T. Konishi, H. Sakurai, and Y. Ohta, J. Phys. Soc. Japan 86, 033701 (2017).
  - [2] J. Matsuno, Y. Okimoto, M. Kawasaki, and Y. Tokura, Phys. Rev. Lett. 95, 176404 (2005).
  - [3] J. Jeanneau, P. Toulemonde, G. Remenyi, A. Sulpice, C. V. Colin, V. Nassif, E. Suard, F.c Gay, R. Weht, and M. Núñez-Regueiro, Euro. Phys. Lett. 127, 27002 (2019).
  - [4] D. I. Khomskii, *Transition Metal Compounds*, Cambridge University Press (2014).

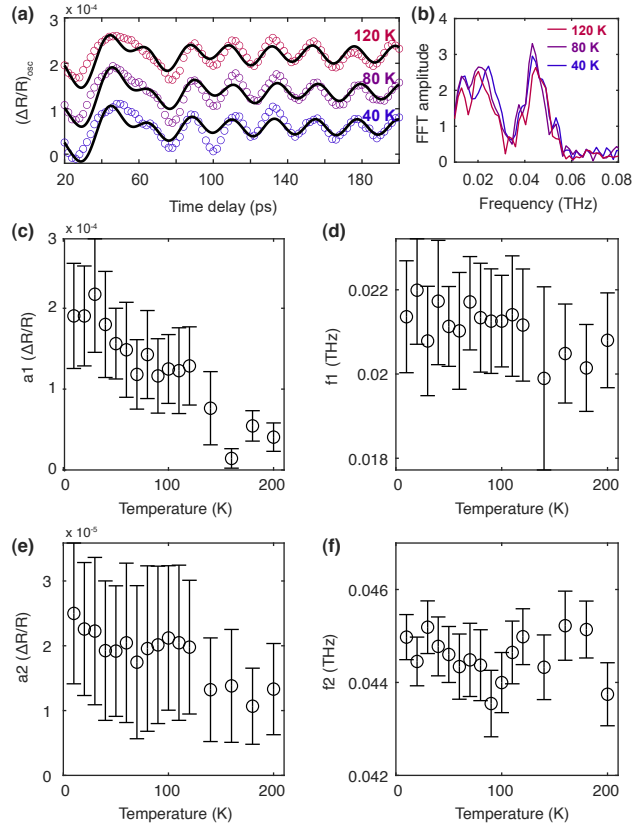

FIG. S7. Coherent acoustic phonon oscillations in  $\text{Sr}_2\text{CrO}_4$ . (a) The oscillatory signals originating from acoustic phonons observed in the transient reflectivity signal after subtracting the electronic responses by means of an exponential decay fit. (b) Fourier transform of the oscillations. (c-f) The amplitudes ( $a_1$  and  $a_2$ ) and frequencies ( $f_1$  and  $f_2$ ) of the two acoustic phonon modes extracted from a damped harmonic oscillator model fit.
